# Supplementary material for: Implantation and atomic scale investigation of self-interstitials in graphene
Source: arXiv:1407.3071 source file (2015-01-16)
Supplement: Supplementary file 1 [file supplementary_information.pdf]

# Implantation and atomic scale investigation of self-interstitials in graphene: Supplementary figures

Ossi Lehtinen, Nilesh Vats, Gerardo Algara-Siller, Pia Knyrim, and Ute Kaiser

*Central Facility for Electron Microscopy, Group of Electron Microscopy of Materials Science, Ulm University, Germany*

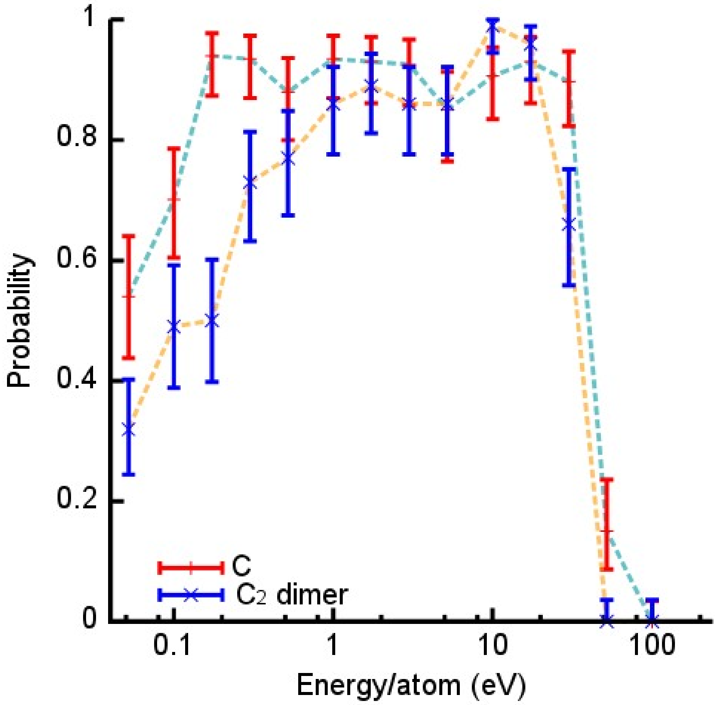


**Supplementary figure 1 | Probability of an incoming C atom and C2 dimer to bond to graphene as a function of kinetic energy.** For each data point 100 individual impacts of incoming C atoms or dimers at random positions were simulated. An event was determined to result in bonding if the incoming atom or one/both of the dimer atoms was bonded to the lattice, and no other atom was sputtered as a result of the impact. The confidence intervals are calculated using the Clopper-Pearson method and represent the 95% interval. The dashed lines are guides to the eye.

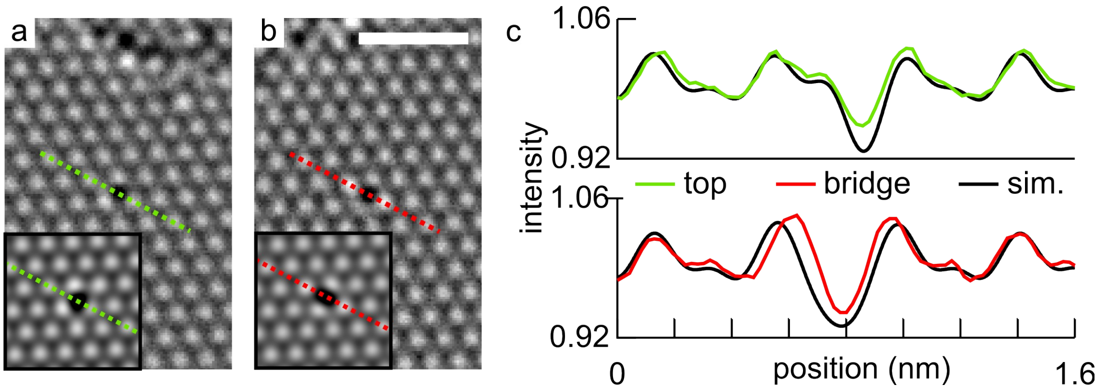


**Supplementary figure 2 | Contrast analysis of the dark spots observed by AC-HRTEM in single layer graphene after carbon deposition.** **a**: A dark spot positioned on top of a carbon atom in graphene. The inset shows a simulated image of a carbon adatom positioned above a carbon atom in graphene (in a projected HRTEM image it cannot be distinguished, whether the extra atom is elevated above graphene, or if the atoms are in the dumbbell configuration [1]). **b**: A dark spot positioned above a C-C bond (the bridge position [2]). The inset shows a simulated image of a carbon adatom in the bridge position. **c**: Measured and simulated intensity profiles across the dark spots. (Fig. 1 b). Intensity profiles across the dark spots in the experimental and simulated HRTEM micrographs show good agreement. According to theoretical calculations, the most stable position is at the bridge site [3], with the top site being slightly less stable [4]. Adatoms on graphene have been predicted to have a migration barrier of 0.47 eV [3], which would imply rapid diffusion at room temperature, while the dark spots are observed to be remarkably stable even under the electron beam. Thus, we conclude that the spots are likely other types of defects, such as adsorbed molecules like CH3 [5] or even silicon in a substitutional position [6].

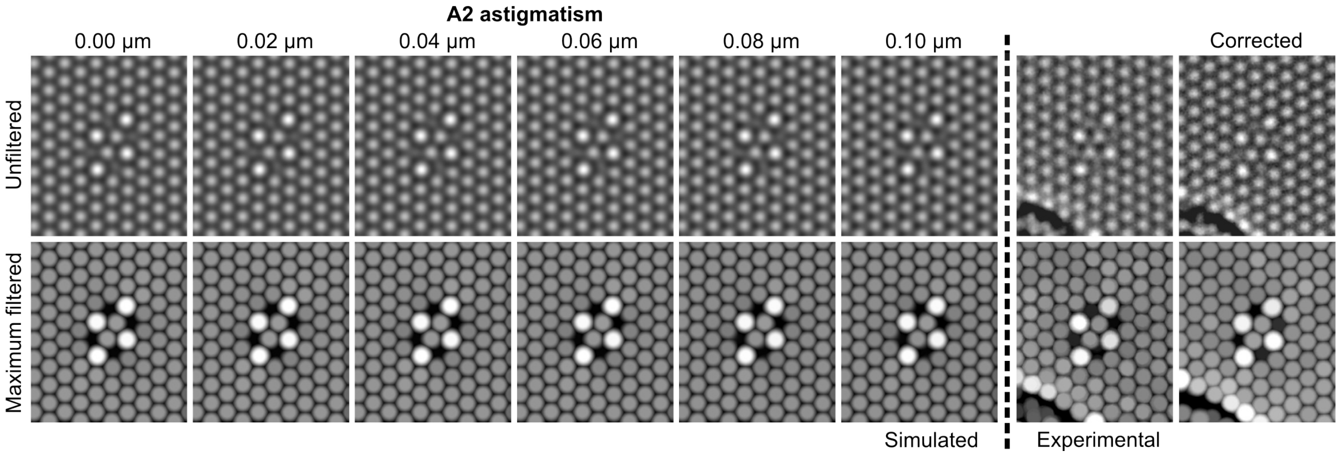


**Supplementary figure 3 | A comparison of simulated and experimental HRTEM images of a self-interstitial with residual A2 astigmatism.** The upper row shows the unfiltered images, and the lower row the same images after maximum filtering [7]. The six left side columns simulated images of the reconstructed self-interstitial with an increasing amount of A2 astigmatism. The second to last column shows a real HRTEM image of the same defect, where residual aberrations are present (the effect matches what is seen in the simulation and thus the dominant aberration can be identified as A2 in the experimental image). As can be seen, the maximum filtered images are not affected by the A2 astigmatism, and the simulated and real images match perfectly at A2 astigmatism of 0.10 µm. The structure can be clearly and unambiguously identified. In the case of a weak scattering object (such as graphene at 80 kV), the effect of residual geometric aberrations, like the three-fold A2 astigmatism can be numerically corrected in the recorded images [8]. The last column in the figure shows the experimental HRTEM image after such correction, where the resulting image matches the simulated image with zero A2 in the first column.

**Supplementary References**


[1] Tsetseris, L.; Pantelides, S. *Carbon* 2009, 47, 901 – 908.

[2] Banhart, F.; Kotakoski, J.; Krasheninnikov, A. V. *ACS Nano* 2011, 5, 26 – 41.

[3] Lehtinen, P. O.; Foster, A. S.; Ayuela, A.; Krasheninnikov, A.; Nordlund, K.; Nieminen, R. M. *Phys. Rev. Lett.* 2003, 91, 017202.

[4] Ma, Y. *Phys. Rev. B* 2007, 76, 075419.

[5] Erni, R.; Rossell, M. D.; Nguyen, M.-T.; Blankenburg, S.; Passerone, D.; Hartel, P.; Alem, N.; Erickson, K.; Gannett, W.; Zettl, A. *Phys. Rev. B* 2010, 82, 165443.

[6] Zhou, W.; Kapetanakis, M. D.; Prange, M. P.; Pantelides, S. T.; Pennycook, S. J.; Idrobo, J.-C. *Phys. Rev. Lett.* 2012, 109, 206803.

[7] Lehtinen, O.; Kurasch, S.; Krasheninnikov, A. V.; Kaiser, U. *Nature Comms.* 2013, 4, 2098.

[8] Lehtinen, O.; Geiger, D.; Lee, Z.; Whitwick, M. B.; Chen, M.-W.; Kis, A.; Kaiser, U. *Ultramicroscopy* 2014, doi:10.1016/j.ultramic.2014.09.010.
